# Supplementary material for: Two-qubit controlled-PHASE Rydberg blockade gate protocol for neutral atoms via off-resonant modulated driving within a single pulse
Source: arXiv:1812.03822 source file (2019-10-18)
Supplement: Supplementary file 1 [file duet_suppl_b1b.pdf]

# Supplemental Material:
# Two-qubit controlled-PHASE Rydberg blockade gate protocol via off-resonant modulated driving within a single pulse

Yuan Sun,[1,2,*] Peng Xu,[3,4] and Ping-Xing Chen[2]

[1] *Key Laboratory of Quantum Optics and Center of Cold Atom Physics, Shanghai Institute of Optics and Fine Mechanics, Chinese Academy of Sciences, Shanghai 201800, China*
[2] *Interdisciplinary Center for Quantum Information, National University of Defense Technology, Changsha 410073, China*
[3] *State Key Laboratory of Magnetic Resonance and Atomic and Molecular Physics, Wuhan Institute of Physics and Mathematics, Chinese Academy of Sciences – Wuhan National Laboratory for Optoelectronics, Wuhan 430071, China*
[4] *Center for Cold Atom Physics, Chinese Academy of Sciences, Wuhan 430071, China*

(Dated: October 18, 2019)

* email: sunyuan17@nudt.edu.cn

This supplementary material is organized as the following. (I) The optimization procedure to compute the appropriate waveform. (II) More details about the two-atom dark state adiabatic driving mechanism. (III) Derivations about the handling of phase modulation. (IV) More information on the performance of the gate, including when it is subject to cold atom's residual thermal motion. (V) Sample calculation of 250 ns phase gate. (VI) Asymmetric driving process due to systematic in-accuracy.

## I. PROCEDURE TO CALCULATE WAVEFORMS

In this section we discuss more details of the tactics to retrieve the appropriate waveforms to arrive at appropriate C-Z gate operation.

We start with the heuristic approach which serves as the precursor for our formal treatment under the framework of off-resonant modulated driving. It comes from a very elementary observation on the time evolution with respect to the two-level atom dressed states, when the atom is driven by modulated optical pulse. Namely, while neglecting non-adiabaticity, what the time evolution brings about can be recognized as phase accumulations on dressed states. Therefore, as long as the dressed states take the same form at the beginning and end, this heuristic approach will simply regard the effect caused by the atom-light interaction as a phase change. More specifically, for given Rabi frequency $\Omega_a$ and detuning $\delta_a$, the interaction Hamiltonian matrix in the rotating wave frame, the dressed states energies, and the corresponding dressed states expressions are as the following:

$$\frac{1}{2}\begin{bmatrix} 0 & \Omega_a \\ \Omega_a^* & 2\delta_a \end{bmatrix},\ \lambda_{+,-} = \frac{1}{2}\delta_a \pm \frac{1}{2}\sqrt{|\Omega_a|^2+\delta_a^2};\ \lambda_+ \sim \begin{bmatrix} \sin\theta e^{-i\varphi} \\ \cos\theta \end{bmatrix},\ \lambda_- \sim \begin{bmatrix} \cos\theta e^{-i\varphi} \\ -\sin\theta \end{bmatrix}. \quad (1)$$

where $\hbar\lambda_{+,-}$ are the dress states' energies, or the so-called adiabatic energies; $\tan(2\theta) \equiv |\Omega_a|/\delta_a$ with $0 \leq \theta \leq \pi$ and $\varphi = \arg(\Omega_a)$. More details can be found at standard atomic physics textbooks.

Therefore, under this very intuitive observation, in order to simultaneously meet the requirement of returning full population to initial state and acquiring a proper phase change, I would like to impose two straightforward conditions: (1) $\Omega_a(t)$ takes the same value at the beginning and ending moments, and so is $\delta_a(t)$; (2) two dressed states accumulate the same phase under the adiabatic assumption $\Phi_d(\Omega_a, \delta_a) = \int \lambda_+(\Omega_a, \delta_a)dt = \int \lambda_-(\Omega_a, \delta_a)dt + 2N\pi, N = 1, 2, 3\ldots$, and the accumulated phase $\Phi_d$ will correspond to gate protocol's demands.

In the above formalism, the Rabi frequency $\Omega_a$ corresponds to the case of $|10\rangle \leftrightarrow |1r\rangle$, $|01\rangle \leftrightarrow |r1\rangle$, while the Rabi frequency $\sqrt{2}\Omega_a$ corresponds to the case of $|00\rangle \leftrightarrow (|r0\rangle + |0r'\rangle)/\sqrt{2}$ assuming perfect Rydberg blockade. With all these understandings, in order to meet the requirement of C-Z gate, one of the simplest forms of the condition imposed by this heuristic approach may be expressed as:

$$\Phi_d(\Omega_a, \delta_a) = 3\pi,\ \Phi_d(\sqrt{2}\Omega_a, \delta_a) = 4\pi. \quad (2)$$

When the smooth waveforms of $\Omega_a, \delta_a$ are described by a set of discrete parameters $x_1, x_2, x_3\ldots$, the constraint of Eq. (2) turns into a set of equations which may be solved numerically. Nevertheless, due to the existence of non-adiabaticity, the waveforms computed by this heuristic approach do not yield the desired high-fidelity gate performance.

However, the basic principle behind the heuristic approach is appealing, where the ultimate goal is to construct a C-Z gate via a single modulated pulse with specially tailored smooth waveform to gain appropriate phase accumulations. Main advantages of this basic principle include avoiding depositing full population at Rydberg state for a finite gap time, avoiding Ramsey type pulse sequence which may put stringent requirement on ground-Rydberg $T_2^*$ coherence time, while suppressing population leakage error and rotation error. The hope is to try overcoming the hurdles by resorting to helpful ideas of adiabatic rapid passage and numerical optimization methods, and this is exactly what we do next for the main purpose of this research effort.

Since we want to employ the tool of numerical methods, this naturally implies that the essentially continuous waveforms need to be represented by a set of discrete parameters such that they may be handled. And therefore we need to carry out a procedure of 'continuous to discrete', for which purpose the Fourier series and Bernstein polynomials float as ideal choices. From mathematical point of view, expansion of Fourier series or Bernstein polynomials form a complete basis for non-pathological functions defined on a finite time interval. Yet on practical account only a limited amount of terms in the expansion will be enough to compute a reasonable waveform for the purpose of gate protocol.

More specifically, we'd like to demonstrate more details here about the process of constructing waveforms for high fidelity gate protocol via resorting to Bernstein polynomials. A Bernstein polynomial is formed from the linear combination of Bernstein basis polynomials, and it becomes the building block of Bézier curves which is important in

modern computer graphics.

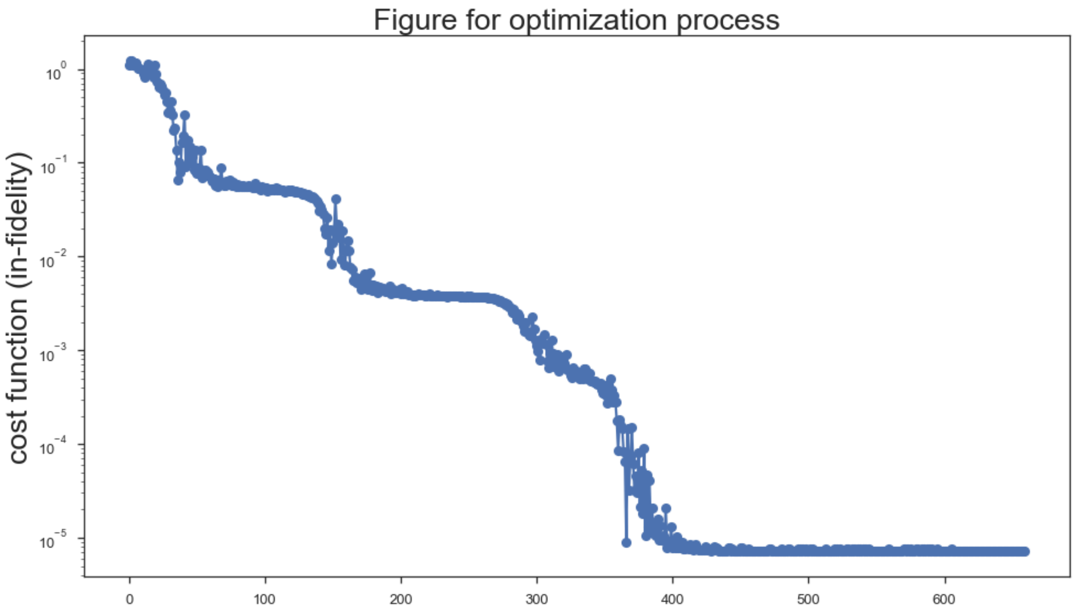


FIG. 1: A typical example of the waveform calculation process, via down-hill simplex numerical optimization method. Horizontal axis represents the index of iterations, while the vertical axis is for the value of cost function in log scale. As the general form of Eq. (5), the amplitude waveform is chosen as $\sum_{\nu=1}^{4}\beta_\nu\left(b_{\nu,n}(t/T_g)+b_{n-\nu,n}(t/T_g)\right)$ where we fix $n=8$, and therefore the waveform is symmetric. The optimization process does not consume too much computation resource and converges quickly. The initial values are set as $\beta_1=1,\beta_2=2,\beta_3=10,\beta_4=6,\Delta_0=-1$ while the calculated result is $\beta_1=1.129,\beta_2=0,\beta_3=4.801,\beta_4=15.038,\Delta_0=-4.019$; all coefficient units are MHz. This example is for the amplitude-only modulation waveform.

For an integer $n$, the $n+1$ Bernstein basis polynomials of degree $n$ is defined on interval $[0,1]$ as the following:

$$b_{\nu,n}(x)=\binom{n}{\nu}x^\nu(1-x)^{n-\nu},\ \nu=0,\ldots,n; \tag{3}$$

where $\binom{n}{\nu}=\frac{n!}{(n-\nu)!\nu!}$ is the binomial coefficient. Then, a Bernstein polynomial may be expressed in terms of the basis polynomials as the following form:

$$B_n(x)=\sum_{\nu=0}^{n}\beta_\nu b_{\nu,n}(x), \tag{4}$$

where $\beta_\nu$'s are real-value coefficients.

On practical account for experimental implementation, it is natural to hope for the amplitude of modulated waveform to start and end at zero, in order to avoid the sharp edge of sudden switching. One convenient feature of is that for $\nu\neq 0,n$, the value of $b_{\nu,n}(x)$ at the end points $0,1$ is exactly zero. Therefore, it is convenient to aim for a truncated form of liner combinations as $B_n(x)=\sum_{\nu=1}^{n-1}\beta_\nu b_{\nu,n}(x)$ with respect to degree $n$, for the purpose of off-resonant driving with only amplitude modulation. That is, the candidate laser waveform may be expressed as:

$$\Omega_s(t)=\sum_{\nu=1}^{n-1}\beta_\nu b_{\nu,n}(t/T_g);\ \Delta(t)=\Delta_0\equiv\ \textit{constant}; \tag{5}$$

where the gate process is defined on time interval $[0,T_g]$.

Starting from Eq. (5), the task turns into finding a set of values $\beta_\nu$ that will yield adequate fidelity with respect to the C-Z gate requirement. Instead of an analytic method, we decide to resort to numerical optimization algorithms. And later on it turns out that the down-hill simplex method, also known as Nelder-Mead algorithm, performs particularly

well for our purpose. The cost function is chosen naturally as the in-fidelity $1-F$evaluated at the end time $t=T_g$ for the two-atom system. Meanwhile, during the optimization process, we keep the positiveness $\Omega_s(t)>0$ all the time since if negative value of $\Omega_s(t)$ occurs on $t\in[0,T_g]$ it means a sudden phase change of the optical field, which is a pathological situation. The evolution of cost functions over iterations of optimization in a sample calculation is shown in Fig. 1.

The calculation procedure for the case of both amplitude and phase modulations is similar, with the exception that Fourier series is adopted instead of the Bernstein polynomial, and we skip the details here. We regard the modulation waveform calculated above as a special example. Moreover, we believe that the choice of expansion basis is not unique and there exist many different types of waveforms that will satisfy the purpose. We anticipate that the deep learning algorithms will further improve this process of calculating appropriate waveforms.

## II. TWO-ATOM DARK STATE

Ref. [1] provides a nice introduction of the two-atom dark state technique and how it helps to suppress the rotation error. Nevertheless, since the situation with our gate protocol is different from the typical $\pi$–gap–$\pi$ framework of Ref. [1], we would like to offer more explanations on the underlying physical mechanism here.

When the two qubits start in states of $|01\rangle$ or $|10\rangle$, it only probes the ground-Rydberg transition in a straightforward manner. The Förster resonance structure will only be accessed when the initial state becomes $|00\rangle$, and this is exactly where the dark state driving mechanism may play an essential role. Main advantages include eliminating the rotation error and lowering the requirement on blockade strength.

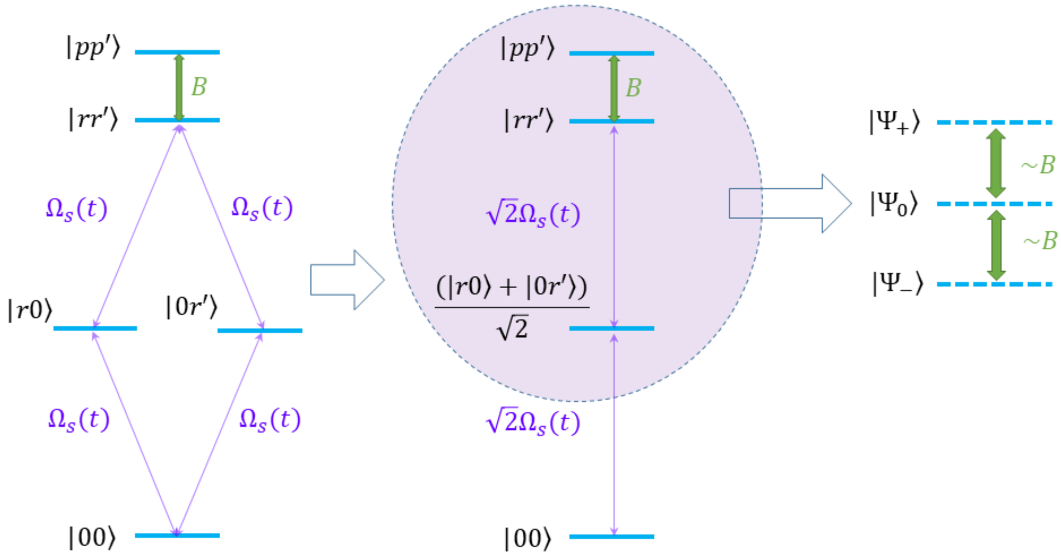


FIG. 2: Schematic of atomic levels of the dark state mechanism for the Rydberg phase gate under investigation, including the Förster resonance structure. The coupling between $|00\rangle$ and $(|r0\rangle+|0r'\rangle)/\sqrt{2}$ is given by Rabi frequency $\sqrt{2}\Omega_s(t)$ and detuning $\Delta(t)$.

At a first glance, the transition occurs between the launching state $|00\rangle$ and the target state $(|r0\rangle+|0r'\rangle)/\sqrt{2}$ (which will again be denoted as $|R\rangle$ to keep a succinct notation) under the idealized situation of perfect Rydberg blockade. Nevertheless, after taking the details of linkage structure into consideration as shown in Fig. 2, the situation of the target state becomes a consequence of the interactions between $|R\rangle$, $|rr'\rangle$ and $|pp'\rangle$. For simplicity we'd like to assume that the energy penalty term $\delta_p$ is zero. Therefore, the Hamiltonian for this system under the rotating wave approximation can be put down as the following matrix form:

$$\mathcal{H}=\hbar\begin{bmatrix}-\Delta & \frac{\sqrt{2}}{2}\Omega_s & 0\\ \frac{\sqrt{2}}{2}\Omega_s^* & 0 & B\\ 0 & B^* & 0\end{bmatrix} \tag{6}$$

For our case, it is customary to have $|\Omega_s|\ll|B|$ and $|\Delta|\ll|B|$ and therefore it makes sense to check the situation

with expansion up to 1st order in $|\Omega_s|/|B|$ and $|\Delta|/|B|$. The energy eigenvalues are:

$$\Delta_0 = -\Delta,\, \Delta_+ = |B|(1+\frac{|\Omega_s|^2}{4|B|^2}),\, \Delta_- = -|B|(1+\frac{|\Omega_s|^2}{4|B|^2}); \tag{7}$$

with the corresponding eigenstates listed below:

$$|\Psi_0\rangle = \cos\beta_2\cos\beta_3|R\rangle + \cos\beta_2\sin\beta_3|rr'\rangle - \sin\beta_2|pp'\rangle, \tag{8a}$$

$$|\Psi_+\rangle = (\sin\beta_1\sin\beta_2\cos\beta_3 - \cos\beta_1\sin\beta_2)|R\rangle + (\cos\beta_1\cos\beta_3 + \sin\beta_1\sin\beta_2\sin\beta_3)|rr'\rangle + \sin\beta_1\cos\beta_2|pp'\rangle, \tag{8b}$$

$$|\Psi_-\rangle = (\cos\beta_1\sin\beta_2\cos\beta_3 + \sin\beta_1\sin\beta_2)|R\rangle + (-\sin\beta_1\cos\beta_3 + \cos\beta_1\sin\beta_2\sin\beta_3)|rr'\rangle + \cos\beta_1\cos\beta_2|pp'\rangle; \tag{8c}$$

while the angles of $\beta_1, \beta_2, \beta_3$ are defined as:

$$\tan\beta_1 = 1,\, \tan\beta_2 = -\frac{2\sqrt{2}|\Omega_s||B|}{\sqrt{2\Delta^2\Omega_s^2 + (\Delta^2 - 4B^2)^2}},\, \tan\beta_3 = -\frac{\sqrt{2}\Omega_s\Delta}{\Delta^2 - 4|B|^2}; \tag{9}$$

where the expressions hold up to 1st order.

In particular, we want to take a closer look at $|\Psi_0\rangle$, which is the dark state coupling to $|00\rangle$. Up to 1st order, in fact $\sin\beta_3 \approx 0$. Therefore $|\Psi_0\rangle$ only practically contains components from $|R\rangle$ and $|pp'\rangle$. For the case of smoothly modulated pulse where $\Omega_s(t)$ starts and ends at zero value, $|\Psi_0\rangle$ coincides with $|R\rangle$ at the beginning and ending moments and thereby no significant amount population is left on the doubly excited Rydberg states after the gate protocol. Due to this effect and the fact that $\Delta_0$ stays stable at the value of $-\Delta$ up to 1st order throughout the interaction process, the dark state mechanism eliminates the rotation error.

During this interaction process, adiabatic following plays an essential role to ensure the validity of dark state mechanism, and therefore it requires that the pulse waveform is sufficiently small and smooth to prohibit the influences of $|\Psi_+\rangle, |\Psi_-\rangle$. In other words, the condition may be stated as $|B| \cdot t_c \gg 1$ together with $(\Omega_{s0}/|B|)^2 \ll 1$ or simply $\Omega_{s0} \ll |B|$, where $t_c$ is the characteristic gate time and $\Omega_{s0}$ is the mean amplitude of the waveform $\Omega_s(t)$. With respect to experimentally practical Rydberg blockade strength and laser parameters, this condition may be well satisfied.

## III. PHASE MODULATION

The first errand right here aims at resolving the subtle details of handling frequency modulation in atom-light interaction. I'd like to begin with an EOM with respect to a rotating wave frame defined in a usual manner:

$$i\frac{d}{dt}\begin{bmatrix} C_0 \\ C_r \end{bmatrix} = \begin{bmatrix} 0 & \frac{1}{2}\Omega_s e^{i\frac{\theta}{\delta}\sin(\delta t)} \\ \frac{1}{2}\Omega_s e^{-i\frac{\theta}{\delta}\sin(\delta t)} & \Delta \end{bmatrix} \cdot \begin{bmatrix} C_0 \\ C_r \end{bmatrix}. \tag{10}$$

Afterwards, I will move one step further on top of the usual rotating phase, namely:

$$C_{r:\text{old}} = e^{-i\frac{\theta}{\delta}\sin(\delta t)} C_{r:\text{new}}; \tag{11}$$

which does not involve the phase of $C_0$; and this transforms the EOM for $C_{r:\text{new}}$ as:

$$i\frac{d}{dt}\begin{bmatrix} C_0 \\ C_r \end{bmatrix} = \begin{bmatrix} 0 & \frac{1}{2}\Omega_s \\ \frac{1}{2}\Omega_s & \Delta - \theta\cos(\delta t) \end{bmatrix} \cdot \begin{bmatrix} C_0 \\ C_r \end{bmatrix}. \tag{12}$$

In the above Eq. (12), intensity modulation (i.e. amplitude modulation) may also be incorporated as $\Omega_s \equiv \Omega_s(t)$ for real valued $\Omega_s$. More generally, for:

$$i\frac{d}{dt}\begin{bmatrix} C_0 \\ C_r \end{bmatrix} = \begin{bmatrix} 0 & \frac{1}{2}\Omega_s e^{i\Theta(t)} \\ \frac{1}{2}\Omega_s e^{-i\Theta(t)} & \Delta \end{bmatrix} \cdot \begin{bmatrix} C_0 \\ C_r \end{bmatrix}; \tag{13}$$

I may define: $C_{r:\text{old}} = e^{-i\Theta(t)} C_{r:\text{new}}$; and then the EOM of Eq. (13) reduces to:

$$i\frac{d}{dt}\begin{bmatrix} C_0 \\ C_r \end{bmatrix} = \begin{bmatrix} 0 & \frac{1}{2}\Omega_s \\ \frac{1}{2}\Omega_s & \Delta - \frac{d}{dt}\Theta(t) \end{bmatrix} \cdot \begin{bmatrix} C_0 \\ C_r \end{bmatrix}. \tag{14}$$

Therefore, as long as $\frac{d}{dt}\Theta(t)$ is a linear combination of sinusoidal functions, so is $\Theta(t)$, which will be readily compatible with the experimental hardware of optical phase modulators working in the MHz–GHz range.

## IV. PERFORMANCE UNDER REALISTIC IMPERFECTIONS

In this section, we further explore the performance of the gate, especially when it is subject to realistic imperfections commonly encountered in experimental investigations, including the influences of Rydberg states' spontaneous emissions, amplitude fluctuations in the laser pulse, and residual thermal motion of the cold atoms.

To incorporate spontaneous emissions of Rydberg states into the calculation, the decay rate of $|r\rangle, |r'\rangle$ is set as $\gamma_r$, while the decay rate of $|p\rangle$ and $|p'\rangle$ is set as $\gamma_p$. Moreover, to emulate technical noises such as random fluctuations on the amplitude, we set the Rabi frequency as $\Omega_s(t) + W \cdot \Omega_n$, where $W$ takes random values in each MCWF trajectory uniformly distributed between 0 and 1. The corresponding numerical results for time evolution are shown in Fig. 3.

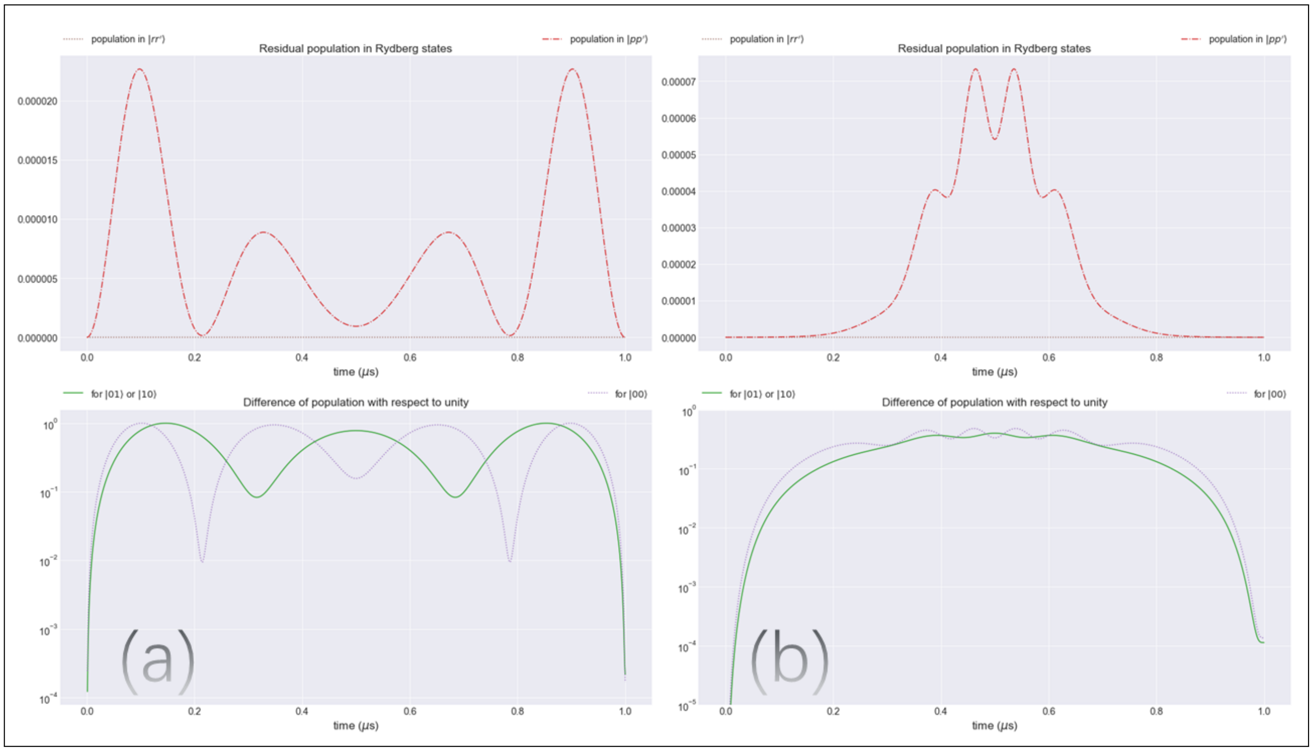


FIG. 3: More details about the performance of modulated waveforms, with the emphasis on the Rydberg population and spontaneous emission's effects. The simulation is for the time evolution of input state $|00\rangle$, averaged over 1 million MCWF trajectories. The settings are $\gamma_r = \gamma_p = \Omega_n = 2\pi \times 0.1$kHz. Here, parameter settings are kept the same as stated in main text, with the extra considerations for spontaneous emission from Rydberg levels and amplitude fluctuations. (a) Waveform with both amplitude and phase modulations defined as: $\Omega_s(t) = \Omega_0 + \Omega_1 \cos(2\pi t/T_g) + \Omega_2 \sin(\pi t/T_g), \Delta(t) = \Delta_0 + \Delta_1 \cos(2\pi t/T_g) + \Delta_2 \sin(\pi t/T_g)$, corresponding to Fig. 2 of main text. The bottom figure shows that the population return with an error on the order of $\sim 10^{-4}$ after interaction. Apparently, the population of $|rr'\rangle$ remains negligible throughout the interaction. (b) Waveform with only amplitude modulation defined as: $\Omega_s(t) = \sum_{\nu=1}^{4} \beta_\nu \left(b_{\nu,n}(t/T_g) + b_{n-\nu,n}(t/T_g)\right), \Delta(t) = \Delta_0 \equiv$ *constant*, corresponding to Fig. 3 of main text. Again, we observe that the population of $|rr'\rangle$ remains negligible throughout the interaction.

The time evolution in Fig. 3 is computed via MCWF methods [2], and we sketch the procedure here. As stated in the main text, we let $|R\rangle = (|r0\rangle + |0r'\rangle)/\sqrt{2}$ denote the single-excitation Rydberg state connected with the ground state $|00\rangle$ via the optical driving field. The starting point is the set of equations of motions without considering the

spontaneous emissions, namely finite line-width of the Rydberg levels:

$$i\frac{d}{dt}\begin{bmatrix}C_0\\C_r\end{bmatrix}=\begin{bmatrix}0 & \frac{1}{2}\Omega_s\\ \frac{1}{2}\Omega_s^* & \Delta\end{bmatrix}\cdot\begin{bmatrix}C_0\\C_r\end{bmatrix};\, i\frac{d}{dt}\begin{bmatrix}X_0\\X_R\\X_{rr'}\\X_{pp'}\end{bmatrix}=\begin{bmatrix}0 & \frac{\sqrt{2}}{2}\Omega_s & 0 & 0\\ \frac{\sqrt{2}}{2}\Omega_s^* & \Delta & \frac{\sqrt{2}}{2}\Omega_s & 0\\ 0 & \frac{\sqrt{2}}{2}\Omega_s^* & 2\Delta & B\\ 0 & 0 & B & 2\Delta+\delta_p\end{bmatrix}\cdot\begin{bmatrix}X_0\\X_R\\X_{rr'}\\X_{pp'}\end{bmatrix}; \tag{15}$$

where $C_0, C_r$ are for the dynamics associated with initial state $|10\rangle$ or $|01\rangle$ and $X_0, X_R, X_{rr'}, X_{pp'}$ are for the dynamics associated with $|00\rangle$. Then the decays may be built into the numerical evaluation by the means of quantum jumps. For a small time interval $\Delta t$, the probability of detecting spontaneous emission from $|r0\rangle$ or $|0r'\rangle$ is $\gamma_r \times \Delta t \times |C_r|^2$, the probability for $|R\rangle$ is $\gamma_r \times \Delta t \times |X_R|^2$, the probability for $|rr'\rangle$ is $2\gamma_r \times \Delta t \times |X_{rr'}|^2$, and the probability for $|pp'\rangle$ is $2\gamma_p \times \Delta t \times |X_{pp'}|^2$. If quantum jumps from the atomic spontaneous emissions do take place, then the atomic state is dragged into the specific eigenstates among the ground level, and we treat it effectively as the atomic population is lost outside of the system under consideration for practical numerical evaluation regarding gate fidelity. Note that one spontaneously emitted single-photon pulse will terminate the two-atom coherent dynamics since it is the two-qubit gate under study. If quantum jumps do not take place, the corresponding excited-state amplitudes shall be reduced. That is to say, $1-\frac{\gamma_r}{2}\Delta t$ for $C_r$ and $X_R$, $1-\frac{\gamma_r}{\Delta}t$ for $X_{rr'}$, and $1-\frac{\gamma_p}{\Delta}t$ for $X_{pp'}$.

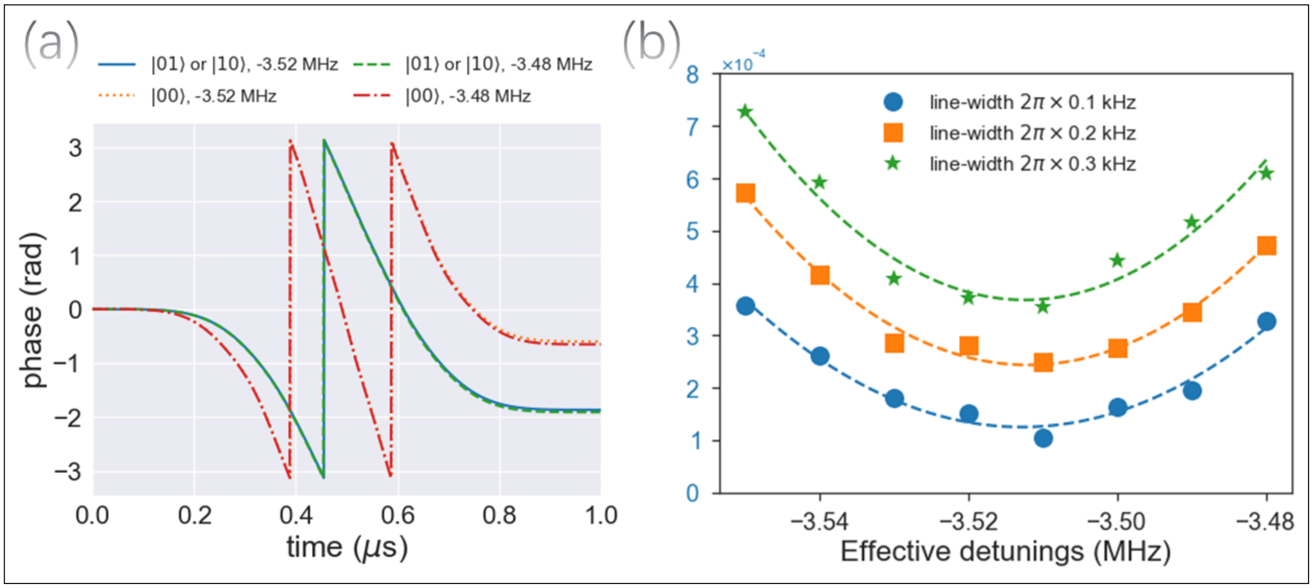


FIG. 4: Information about the performance of gate protocol under influence of detuning offsets, to account for the effects caused by residual thermal motion of the cold atom qubits. The calculations here correspond to the special case where both atoms travel at the same velocity. (a) Phase of the atomic wave function. The $\Delta_0 = -3.48$ MHz curve and $\Delta_0 = -3.52$ MHz curve almost overlap with each other. By the way, the population returns without significant loss. (b) Fidelities with different detuning offsets, each data point is averaged from 0.5 million MCWF trajectories, with settings as $\gamma_r = \gamma_p = \Omega_n = 2\pi \times 0.1$kHz. Fitting to parabolic curve is also included.

Another intrinsic limitation is the residual thermal motion of the qubit atoms. As already been noticed during the experimental efforts with $\pi$–gap–$\pi$ protocol, the atoms' kinematic motion in optical trap constitutes adverse influence to the gate fidelity. This becomes particularly annoying when the ground-Rydberg coupling is driven by the single-photon uv transition, even if the cold atom's thermal velocity is on the order of 1 cm/s – 10 cm/s. Approximately speaking, this detrimental effect is similar to the decoherence of ground-Rydberg Ramsey experiment on an atomic ensemble caused by the velocity distribution.

A typical example is shown in Fig. 4, where we carry out calculations with the same modulated amplitude but different effective detuning $\Delta_0$, in order to emulate the atom-light interaction process for atoms with non-zero velocity for the case of only amplitude modulation. It turns out, the off-resonant modulated driving technique is robust against this imperfection factor. This observation is also related to the fact that this gate protocol achieves necessary operations within a single continuous pulse while does not leave population in the Rydberg state during laser off time. Meanwhile, thanks to the dark state mechanism in the off-resonant modulated driving, even under the presence of detuning offsets, no significant population is left on the doubly excited Rydberg state after interaction.

## V. SAMPLE CALCULATION OF A 250 NANO-SECOND GATE PROCESS

In this section, we discuss a sample calculation of a controlled-PHASE gate whose pulse duration is restricted to 250 ns. The purpose of a shorter pulse duration is to suppress the intrinsic error caused by the spontaneous emission from Rydberg states, which is the major theoretical limit for the off-resonant modulated driving gate protocol.

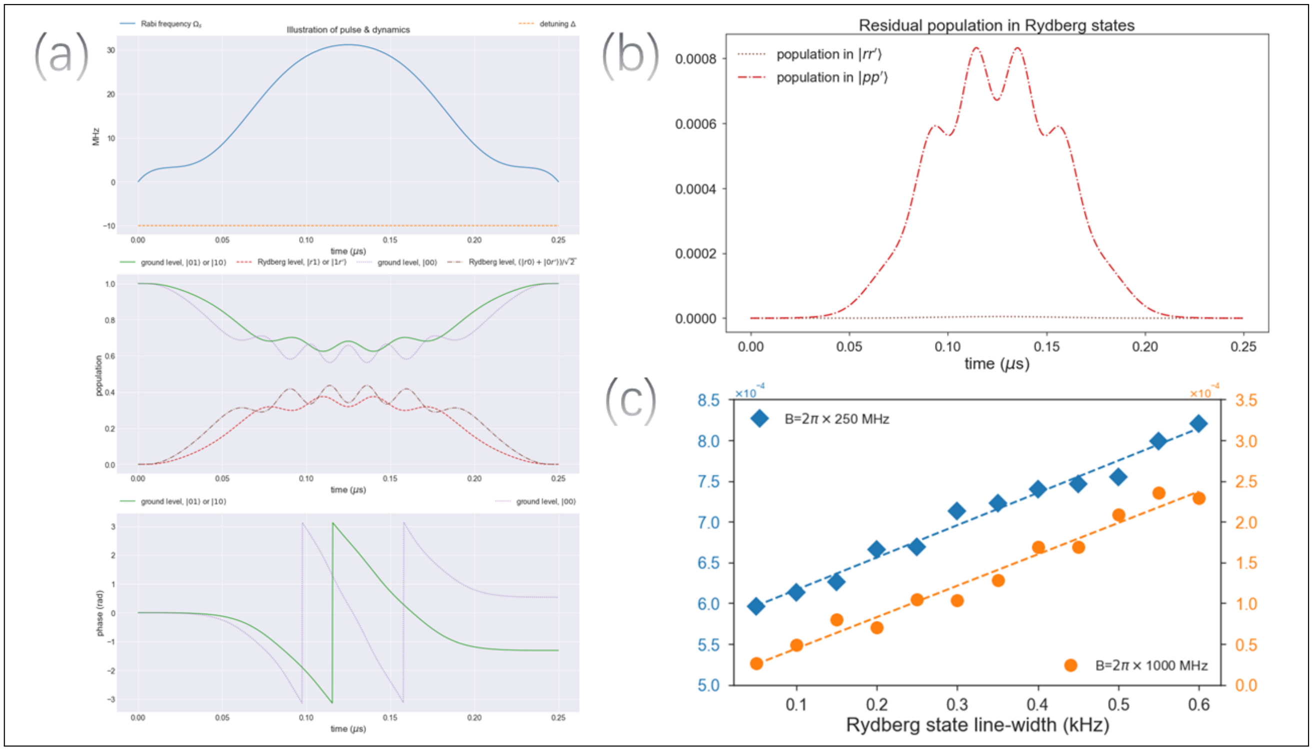


FIG. 5: Numerical results about the performance of a controlled-PHASE gate with time duration of 250 ns. (a) Details of the time evolution, without considering spontaneous emissions. The first graph shows the waveform, the second graph shows the population on different atomic states, while the last graph shows the phase accumulation of the atomic wave function during the atom-light interaction process. (b) Simulation for input state $|00\rangle$ with emphasis on population of Rydberg states during interaction. Similar to the 1 $\mu$s case, the population of $|rr'\rangle$ remains negligible throughout the interaction. The settings are $\gamma_r = \gamma_p = \Omega_n = 2\pi \times 0.1$kHz. (c) Gate fidelities under different conditions, where gate error is plotted against Rydberg decay rates. A local sing-qubit phase rotation is incorporated in the numerical simulation to transform controlled-PHASE gate into a standard C-Z gate. Due to the higher peak Rabi frequency values, it requires relatively stronger Förster resonance strength comparing with the case of 1 $\mu$s gate. Effects of spontaneous emissions and Rabi frequency amplitude fluctuations are considered, and each data point is from averaged evaluations over 0.5 million MCWF trajectories. The amplitude fluctuation is set as $\Omega_n = 2\pi \times 0.1$kHz.

Based upon the waveform calculation techniques presented in Section I, no fundamental difference exists between designing a 1 $\mu$s gate and 250 ns gate. However, from a practical point of view, laser power is not in unlimited supply for experimental apparatus. Therefore, we have designed a slightly different waveform with the intention of mildly suppressing the peak Rabi frequency on top of the previously discussed basic methods. Again, we have obtained a waveform for only amplitude modulation, which is constructed with respect to Bernstein polynomials. Here, the waveform is chosen as $\Omega_s(t) = \sum_{\nu=1}^{8} \beta_\nu \big(b_{\nu,n}(t/T_g) + b_{n-\nu,n}(t/T_g)\big), \Delta(t) = \Delta_0 \equiv$ *constant* with $n = 16$. The relevant parameters include: , $\beta_1 = 7.5308$ MHz, $\beta_2 = 0.6184$ MHz, $\beta_3 = 1.3992$ MHz, $\beta_4 = 0.3316$ MHz, $\beta_5 = 33.6$ MHz, $\beta_6 = 38.4$ MHz, $\beta_7 = 43.0396$ MHz, $\beta_8 = 5.6926$ MHz, $\Delta_0 = -9.96$ MHz and $T_g = 0.25$ $\mu$s. The numerical simulation of the gate performance is presented in Fig. 5, which demonstrates that shorter gate time duration helps to enhance gate fidelity, provided the Rydberg-Rydberg interaction strength is adequate.

Another interesting aspect is that, due to relatively larger atom-light detuning setting and shorter interaction time, in principle 250 ns gate becomes more robust against effects caused by residual thermal motion of the cold atom qubits, compared with 1 $\mu$s gate. However, on the other hand, at this moment it seems that the gate time cannot be reduced to an arbitrarily small time interval yet. The reason comes from the reality that Rydberg-Rydberg interaction

strength may not be experimentally enhanced unlimitedly, at a finite atom-atom distance.

## VI. WHEN RABI FREQUENCIES ARE NOT BALANCED DUE TO IMPERFECTIONS

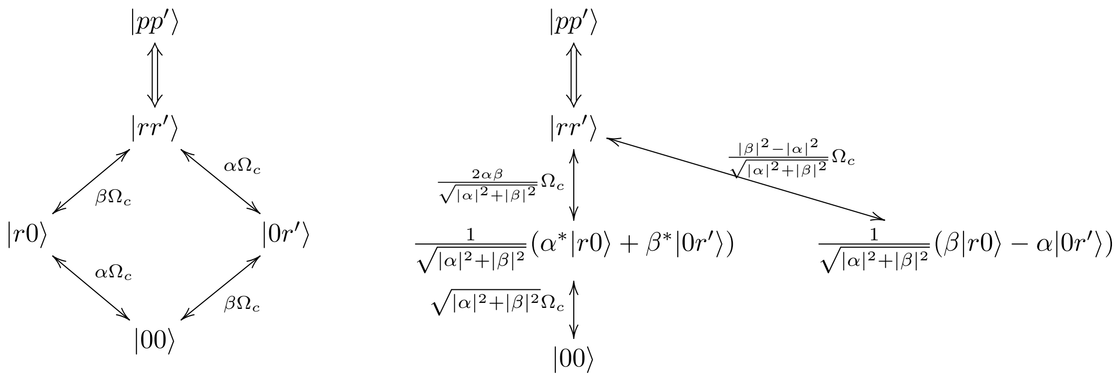


FIG. 6: Transition linkage pattern for the ladder type linkage configuration under consideration, with asymmetric optical driving on two qubit atoms. Morris-Shore transform is employed to show the reduced transition structure and the associated effective Rabi frequencies are also marked. The uncoupled idle state for $|00\rangle$'s ground-Rydberg transition to a singly Rydberg excited state is $(|\alpha|^2+|\beta|^2)^{-1/2}(\beta|r0\rangle-\alpha|0r'\rangle)$; however its transition strength to $|rr'\rangle$ does not vanish and shall be included in a serious calculation.

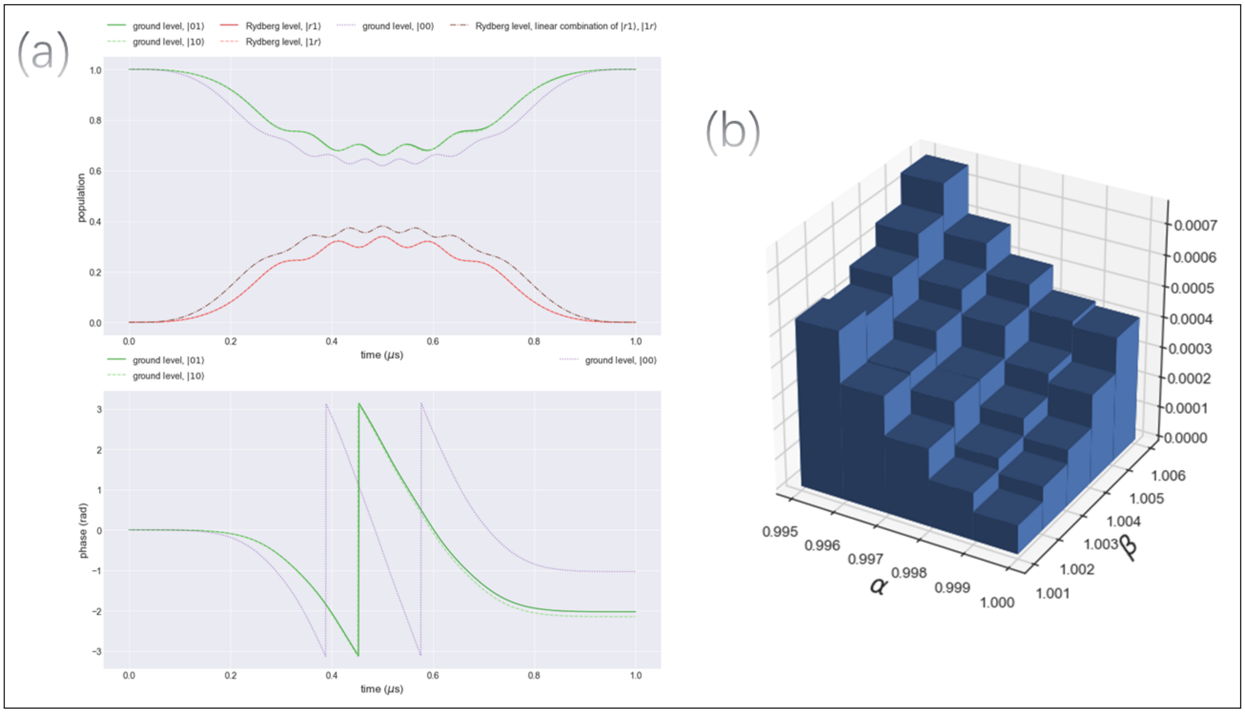


FIG. 7: Information about the performance of gate protocol under the influence of asymmetric driving. (a) Details of the time evolution, without considering spontaneous emissions. The first graph shows the population on different atomic states, while the second graph shows the phase accumulation of the atomic wave function during the atom-light interaction process. (b) Simulation of gate errors under asymmetric driving.

Generally, we only consider it as an idealization to establish a perfect equivalence between the Rabi frequencies

at the sites of the two atomic qubits. Under realistic experimental conditions, the ratio may be set close to 1 but with some minor deviations due to systematic uncertainties, and this ratio may vary shot-to-shot. Therefore, it is reasonable to investigate the gate protocol's performance under such circumstances and estimate its robustness.

We assume that the ideal Rabi frequency is $\Omega_c$, and the actual Rabi frequencies due to asymmetric driving are $\alpha\Omega_c, \beta\Omega_c$ at the two qubit atoms respectively. First of all, the time evolutions of initial state $|01\rangle$ and $|10\rangle$ become different due to asymmetry. Meanwhile, the linkage structure and level configurations involved in the time evolution for initial state $|00\rangle$ are more complicated than the case of perfect symmetric driving, whose details are shown in Fig. 6. Those extra complexities all need to be included in the calculations of the dynamics of the system under study.

Then we carry out numerical simulations to estimate the relevant effects, where a typical sample result is shown in Fig. 7. For Fig. 7(a), we choose the same waveform of only amplitude modulation as the main text and Section IV. In order to clearly demonstrate the influence of the asymmetric driving, the parameters are set as $\alpha = 0.995, \beta = 1.005$ which constitutes a significant deviation from the ideal configuration. For Fig. 7(b), we examine the gate fidelities under different extents of asymmetry and plot the gate error as a function of $\alpha, \beta$. Effects of spontaneous emissions and Rabi frequency amplitude fluctuations are considered, and each data entry is from averaged evaluations over 0.2 million MCWF trajectories. The settings are $\gamma_r = \gamma_p = \Omega_n = 2\pi \times 0.1$kHz.

[1] D. Petrosyan, F. Motzoi, M. Saffman, and K. Mølmer, Phys. Rev. A **96**, 042306 (2017).
[2] J. Dalibard, Y. Castin, and K. Mølmer, Phys. Rev. Lett. **68**, 580 (1992).
